# Supplementary material for: Beyond symmetrization: effective adjacency matrices and renormalization for (un)singed directed graphs
Source: arXiv:2406.01517 source file (2024-06-03)
Supplement: Supplementary file 1 [file curvature.tex]

\begin{equation}
\begin{split}
F_\mathcal G(u, v)= 
w_\mathcal G(u, v)\Bigl(
	w_\mathcal G(v, u)d(u)  -\sum
	d(u)T(v, u)T(u, t)
\Bigl) \\
w_\mathcal G(u, v)\Bigl(
	w_\mathcal G(u, v)d(v)-\sum
	d(v)T(u, v)T(v, r)
\Bigl)
\end{split}
\end{equation}

\begin{equation}
\begin{split}
(F_\mathcal G f)(u, v)= 
f(u)  -w_\mathcal G(u, v)
\sum\limits_{t \in Nei(u)-\{v\}}
T(v, u)T(u, t)f(t) \\
f(v)-w_\mathcal G(u, v)
\sum\limits_{t \in Nei(v)-\{u\}}
T(u, v)T(v, r)f(r)
\end{split}
\end{equation}

não é bom pq queremos que $F(u, v)^\star = F(v, u)$
\begin{equation}
\begin{split}
F_\mathcal G(u, v)&= 
	d(u)  -w_\mathcal G(u, v)
	\sum\limits_{t\in Nei(u)}
		d(u)T(v, u)T(t, u) \\
&+
	d(v)-w_\mathcal G(u, v)
	\sum\limits_{t\in Nei(v)}
		d(v)T(v, u)T(r, v)
\end{split}
\end{equation}
o problema é que $T(r, v)$ e $T(t, u )$ não ficaram simétricos

\begin{equation}
\begin{split}
F_\mathcal G(u, v)&= 
d(u)  -w_\mathcal G(u, v)
\sum\limits_{t\in Nei(u)}
d(u)T(v, u)T(t, u) \\
&+
d(v)-w_\mathcal G(u, v)
\sum\limits_{t\in Nei(v)}
d(v)T(v, u)T(r, v)
\end{split}
\end{equation}

Uma possibilidade é interprestar a raiz do  foreman como modulo do operador $w_\mathcal G$, contudo nesse caso na dilatação até agoran não apareceria nada, pois

$|w_\mathcal G(u, v)w_\mathcal G(t, u)| = w(u, v)w(t, u)$.
\begin{equation}
\begin{split}
F_\mathcal G(u, v)&= 
d(u)  -w_\mathcal G(u, v)
\sum\limits_{t\in Nei(u)}
d(u)T(v, u)\Bigl( T(t, u) + T(u, t) \Bigl ) \\
&+
d(v)-w_\mathcal G(u, v)
\sum\limits_{t\in Nei(v)}
d(v)T(v, u)\Bigl( T(t, u) + T(u, t) \Bigl )
\end{split}
\end{equation}

ainda parece feio , como realacionar com algo??

\begin{equation}
\begin{split}
(F_\mathcal G f)(u, v)&= 
d(u)f(u)  -w_\mathcal G(u, v)
\sum\limits_{t\in Nei(u)}
d(u)T(v, u)\Bigl(T(u, t)f(t) - T(t, u)f(u) \Bigl ) \\
&+
d(v)-w_\mathcal G(u, v)
\sum\limits_{t\in Nei(v)}
d(v)T(v, u)\Bigl(T(v, r)f(r) - T(r, v)f(v) \Bigl )
\end{split}
\end{equation}

\begin{equation}
\begin{split}
(F_\mathcal G f)(u, v)&= 
d(u)f(u)  -w_\mathcal G(u, v)
\sum\limits_{t\in Nei(u)}
d(u)T(v, u)(\mathrm{grad}_\mathcal G f)(u, t) \\
&+
d(v)-w_\mathcal G(u, v)
\sum\limits_{t\in Nei(v)}
d(v)T(v, u)(\mathrm{grad}_\mathcal G f)(v, r)
\end{split}
\end{equation}
