# Supplementary material for: Beyond symmetrization: effective adjacency matrices and renormalization for (un)singed directed graphs
Source: arXiv:2406.01517 source file (2024-06-03)
Supplement: Supplementary file 2 [file graph2graph.tex]

\begin{lemma}[(Un)directed Map from sync]
%[(Un)directed Map from sync]	
	Se $\omega(u,v) =1$ então a frustação mapeia para um grafo não direcionado
	caso contrário direcionado.
	\begin{align}
\xi(u,v)^2=	\parallel\omega(u, v)f(v) - w_\mathcal G(u, v)f(u)\parallel^2
	\nonumber\\
	=\omega(u, v)\omega(u, v)^\star|f(v)|^2 +
	  	w_\mathcal G(u, v)	w_\mathcal G(u, v)^\star|f(u)|^2 +
	  	\nonumber\\
	  -\omega(u, v)w_\mathcal G(u, v)^\star f(v) f(u)^\star
	  -\omega(u, v)^\star w_\mathcal G(u, v)f(v)^\star f(u)\nonumber
	  	\end{align}	
	  Se $\omega(u, v) = 1\, \forall (u, v)$,
	  como $w_\mathcal G(u, v)^\star = w_\mathcal G(v, u)$ e $w_\mathcal G(u, v)w_\mathcal G(v, u) = 1$, seja $|f(u)|^2 = 1$ então
	  \begin{align}
	 \xi(u,v)^2 = 2 
	 	- \left(
	 		f(v)w_\mathcal G(v, u)f(u)^\star 
	 		+f(u) w_\mathcal G(u, v) f(v)^\star
		\right)
	  \end{align}
	  
	  De maneira análoga
	  \begin{align}
	  \xi(v, u)^2 = 2 - \left(
	  f(u)w_\mathcal G(u, v)f(v)^\star 
	  +f(v) w_\mathcal G(v, u) f(u)^\star
	  \right)
	  \end{align}
	  
\end{lemma}

\begin{lemma}[Undirected Map from energy functional]
	O funcional de energia permite mapear todo grafo com potêncial 
	nas arestas em um grafo com função peso simétrica, isto é,
	não direcionado.
	\begin{align}
	\xi^{(T)}(u, v) &= \xi^{(T)}(v, u)
	\end{align}	
	\begin{align}
	T(u, v)f(v) - T(v, u)f(v)
	\end{align}
\end{lemma}
